# Supplementary material for: Towards data-driven stochastic predictive control
Source: arXiv:2212.10663 source file (2022-12-20)
Supplement: Supplementary file 1 [file Sec7_Appendix.tex]

\section*{Appendix}\label{sec:appen}
\subsubsection*{Proof of Proposition \ref{pro:no_truncation_error}}  

The PCEs for $X_k$ and \textit{i.i.d.} noise $W_{k+i}$ are given by
\begin{align*}
	X_k(\omega_x) &= \pce{x}_k^0 \phi_x^0 + \sum_{j=1}^{L_{x}}\pce{x}_k^j  \phi_x^j( \omega_x),\\
W_{k+i}(\omega_i) &= \pce{w}_{k+i}^0\phi_{w_i}^0 + \sum_{j=1}^{L_w}\pce{w}_{k+i}^j\phi_{w_i}^j(\omega_i),
\end{align*}
where $\phi^0_x=\phi_{i}^0=1$ and $\phi_{i}^j(\omega_i),j=1,...,L_w$ are polynomials of independent random variables $\omega_i,i\in \I_{[0,N-1]} $.  We construct a new basis with $L_{x} + NL_w + 1$ terms 
\begin{equation}\label{eq:new_basis}
	\varphi = \begin{bmatrix} 1 & \varphi_{x_k}^\top(\omega) & \varphi_{w_k}^\top(\omega_0)  \cdots  \varphi_{w_{k+N-1}}^\top(\omega_{N-1}) \end{bmatrix}^\top
\end{equation}
\text{with}
\begin{align*}
	\varphi_{x_k}(\omega) &= \begin{bmatrix} \phi^1(\omega) & \cdots & \phi^{L_{x}}(\omega) \end{bmatrix}^\top,\\
	\varphi_{w_{k+i}}(\omega_i) &= \begin{bmatrix} \phi_{w_i}^1(\omega_i) & \cdots & \phi_{w_i}^{L_w}(\omega_i) \end{bmatrix}^\top,
\end{align*}
where  $i\in \I_{[0,N-1]}$. Observe that $X_k$ and $\mbf{W}$ satisfy Definition~\ref{def:exact_pce} in the basis \eqref{eq:new_basis}. Moreover, Assumption \ref{ass:input_disturbance} implies that Definition \ref{def:exact_pce} also holds for $\mbf{U}^\star$. For linear systems \eqref{eq:OCPdynamic}, $\mbf{X}^\star$ is linked to $\mbf{W}$ and $\mbf{U}^\star$ via an affine mapping. Hence the conclusion that $\mbf{X}^\star$ admits an exact PCE under the same basis \eqref{eq:new_basis}, cf. \cite{muehlpfordt18comments}. $\hfill \blacksquare$

\subsubsection*{Derivation of \eqref{eq:causality_input}} 
 Consider the basis~\eqref{eq:new_basis} and the PCEs
\begin{equation}\label{eq:pce_newbasis}
U\pred{i}{k} = \pce{u}\pred{i}{k}^0 + \pce{u}\pred{i,x}{k}^\top \varphi_{x} + \sum_{j=0}^{N-1}\pce{u}\pred{i,w_j}{k}^\top \varphi_{w_j},
\end{equation}
where $\pce{u}\pred{i,x}{k}$ and $\pce{u}\pred{i,w_j}{k}$ denote the PCE coefficients of $U\pred{i}{k},~i\in\set{I}_{[k,k+N-1]}$ corresponding to the basis function $\varphi_{x}$ and $\varphi_{w_j}$ respectively. Then the causality requirement can be formulated as
\begin{equation} \label{eq:causality_pce_newbasis}
	\pce{u}\pred{i,w_j}{k} = 0, \quad j\in \I_{[i-k,N-1]}, \, i \in \I_{[k,k+N-1]}.
\end{equation}
Comparing \eqref{eq:pce_newbasis} to the PCE expression
\[
U\pred{i}{k} = \pce{u}\pred{i}{k}^0 + \sum_{j=1}^{L} \pce{u}\pred{i}{k}^j\phi^j \text{ with } L = L_x + NL_w,
\]
we obtain
\begin{subequations}
	\begin{align*}
		\varphi_{x_k} &= \begin{bmatrix} \phi^1 & \phi^2 &\cdots & \phi^{L_{x}} \end{bmatrix}^\top, \\
		\varphi_{w_j} &= \begin{bmatrix} \phi^{p+1} & \phi^{p+2} &\cdots & \phi^{p+L_w} \end{bmatrix}^\top, \\
		\pce{u}\pred{i,x}{k} &= \begin{bmatrix} \pce{u}\pred{i}{k}^{1} & \pce{u}\pred{i}{k}^{2} &\cdots & \pce{u}\pred{i}{k}^{L_{x}} \end{bmatrix}^\top, \\
		\pce{u}\pred{i,w_j}{k} &= \begin{bmatrix} \pce{u}\pred{i}{k}^{p+1} & \pce{u}\pred{i}{k}^{p+2} &\cdots & \pce{u}\pred{i}{k}^{p+L_w} \end{bmatrix}^\top,
	\end{align*}
\end{subequations}
where $p = L_{x}+jL_w$. Hence~\eqref{eq:causality_pce_newbasis} can be reformulated as
\begin{equation*}
	\pce{u}\pred{i}{k}^{j} = 0, j\in \I_{[L_{x}+(i-k)L_w+1,L]},\, i \in \I_{[k,k+N-1]}.
\end{equation*}
